# Supplementary material for: Efficient B-Spline Finite Elements for Cloth Simulation
Source: arXiv:2506.18867 source file (2026-05-01)
Supplement: Supplementary file 1 [file supp-doc.pdf]

# A B-Spline Finite Element Method for Cloth Simulation

## Supplemental Document

YUQI MENG, Carnegie Mellon University, USA and University of Utah, USA

YIHAO SHI, Carnegie Mellon University, USA and Zhejiang University, China

KEMENG HUANG, Carnegie Mellon University, USA and University of Hong Kong, China

NING GUO, Zhejiang University, China

TAKU KOMURA, University of Hong Kong, China

YIN YANG, University of Utah, USA

MINCHEN LI, Carnegie Mellon University, USA

CCS Concepts: • **Computing methodologies** → **Physical simulation**.

Additional Key Words and Phrases: B-Spline FEM, Cloth Simulation, Membrane Locking, Bending

### CONTENTS

|                                   |   |
|-----------------------------------|---|
| Contents                          | 1 |
| 1 Derivatives of Inverse Function | 1 |
| 2 Derivation of Elasticity Energy | 2 |
| 2.1 Membrane Energy               | 2 |
| 2.2 Bending Energy                | 3 |
| 3 Performance Optimization        | 4 |
| 3.1 Solver Details                | 4 |
| 3.2 Fast Hessian Assembly         | 5 |
| 4 Additional Results              | 6 |
| References                        | 7 |

## 1 Derivatives of Inverse Function

We first derive the (bivariate) inverse function theorem for second order derivatives. The explicit formula is very important for deriving the derivatives of our bending energy, detailed in [subsection 2.2](#). For notational simplicity, we will use subscripts to denote derivatives in the following derivations, e.g.  $u_x := \partial u / \partial x$ ,  $u_{xx} := \partial^2 u / \partial x^2$ .

Given a bijective  $C^2$  vector-valued function  $\mathcal{T} : \mathbb{R}^2 \rightarrow \mathbb{R}^2$ ,  $\mathcal{T}(u, v) = (x(u, v), y(u, v))$ , there exists an (implicit) inverse function of it  $\mathcal{T}^{-1}(x, y) = (u(x, y), v(x, y))$ . Here we use  $u, v, x, y$  to denote both the variable and the function describing correlation. We would like to compute the second order derivatives  $u_{xx}$ ,  $u_{xy}$ ,  $u_{yy}$ , and similar for  $v$ , using only derivatives of  $x, y$  w.r.t.  $u, v$ , which are available from the explicit relations.

Consider the equation

$$u = u(x(u, v), y(u, v)) \tag{1}$$

---

Authors' Contact Information: Yuqi Meng, Carnegie Mellon University, USA and University of Utah, USA; Yihao Shi, Carnegie Mellon University, USA and Zhejiang University, China; Kemeng Huang, Carnegie Mellon University, USA and University of Hong Kong, China; Ning Guo, Zhejiang University, China; Taku Komura, University of Hong Kong, China; Yin Yang, University of Utah, USA; Minchen Li, Carnegie Mellon University, USA, minchernl@gmail.com.

First we compute the first order derivatives of the inverse function. Applying partial derivatives w.r.t. to  $u$  and  $v$  respectively on Equation 1 and applying chain rule gives the following linear system:

$$\begin{cases} u_u = x_u u_x + y_u u_y \\ u_v = x_v u_x + y_v u_y, \end{cases} \quad (2)$$

where the unknowns are highlighted, and left hand sides of the systems evaluate to  $u_u = 1, u_v = 0$ . Solving the system gives the first-order derivatives  $u_x, u_y, v_x$  and  $v_y$ :

$$\begin{cases} u_x = \frac{y_v}{x_u y_v - x_v y_u} \\ u_y = -\frac{x_v}{x_u y_v - x_v y_u}. \end{cases} \quad (3)$$

By symmetry, exchanging  $u$  and  $v$  gives the derivatives of  $v$ .

Now take the second-order derivatives w.r.t.  $x$  and  $y$  on both sides of Equation 1. This gives another linear system where the unknowns are the second-order derivatives:

$$\begin{cases} u_{uu} = x_u^2 u_{xx} + 2x_u y_u u_{xy} + y_u^2 u_{yy} + u_x x_{uu} + u_y y_{uu} \\ u_{vv} = x_v^2 u_{xx} + 2x_v y_v u_{xy} + y_v^2 u_{yy} + u_x x_{vv} + u_y y_{vv} \\ u_{uv} = x_u x_v u_{xx} + (x_u y_v + x_v y_u) u_{xy} + y_u y_v u_{yy} + u_x x_{uv} + u_y y_{uv}. \end{cases} \quad (4)$$

Here left hand side of all three equations evaluate to 0. Solving Equation 4 gives the explicit expression of second order derivatives:

$$\begin{cases} u_{xx} = -\frac{1}{(x_v y_u - x_u y_v)^2} (u_x (x_{uu} y_v^2 - 2x_{uv} y_u y_v + x_{vv} y_u^2) + u_y (y_{uu} y_v^2 - 2y_{uv} y_u y_v + y_{vv} y_u^2)) \\ u_{xy} = -\frac{1}{(x_v y_u - x_u y_v)^2} (u_x (x_{uv} y_v^2 - x_u x_{vv} y_u + x_v x_{uv} y_u - x_v x_{uu} y_v)) + u_y (x_u y_{uv} y_v - x_u y_{vv} y_u + x_v y_u y_{uv} - x_v y_v y_{uu}) \\ u_{yy} = -\frac{1}{(x_v y_u - x_u y_v)^2} (u_x (x_{uu} x_v^2 - 2x_{uv} x_u x_v + x_{vv} x_u^2) + u_y (y_{vv} x_u^2 - 2y_{uv} x_u x_v + y_{uu} x_v^2)). \end{cases} \quad (5)$$

Similarly, exchanging  $u$  and  $v$  gives the derivatives of  $v$ .

## 2 Derivation of Elasticity Energy

In this section we provide the detailed derivation of membrane and bending energy and their derivatives, discretized onto the degrees of freedom (DOFs) of quadratic B-spline surfaces.

### 2.1 Membrane Energy

Recall that in the FEM Baraff-Witkin model [Kim 2020], the membrane energy density  $\Psi_{\text{mem}}$  is defined as the sum of stretching and shearing components

$$\begin{aligned} \Psi_{\text{shear}} &= \mu_{\text{sh}} I_6^2, \\ \Psi_{\text{stretch}} &= \mu_{\text{st0}} \left( \sqrt{I_5(\mathbf{e}_0)} - 1 \right)^2 + \mu_{\text{st1}} \left( \sqrt{I_5(\mathbf{e}_1)} - 1 \right)^2, \end{aligned} \quad (6)$$

using the anisotropic invariants

$$I_5(\mathbf{e}_0) = \mathbf{e}_0^T \mathbf{F}^T \mathbf{F} \mathbf{e}_0, \quad I_5(\mathbf{e}_1) = \mathbf{e}_1^T \mathbf{F}^T \mathbf{F} \mathbf{e}_1, \quad I_6(\mathbf{e}_0, \mathbf{e}_1) = \mathbf{e}_0^T \mathbf{F}^T \mathbf{F} \mathbf{e}_1. \quad (7)$$

All of these invariants are computed using the in-plane deformation gradient  $\mathbf{F}$ , which is computed via treating parametric coordinates as intermediates, and applying chain rule:

$$F_{\alpha\beta} := \frac{\partial \phi_\alpha}{\partial X_\beta} = \sum_{(i,j) \in I} \frac{\partial N_{i,j}}{\partial u} \mathbf{c}_\alpha^{i,j} \frac{\partial u}{\partial X_\beta} + \sum_{(i,j) \in I} \frac{\partial N_{i,j}}{\partial v} \mathbf{c}_\alpha^{i,j} \frac{\partial v}{\partial X_\beta}, \quad (8)$$

where  $\phi$  is the deformation,  $N_{i,j}$  are the quadratic B-spline basis,  $\mathbf{C}^{i,j}$  are the control points,  $(X_\beta)$  are the material space coordinates for  $\beta \in \{1, 2\}$ , and  $(u, v)$  are the parametric coordinates. The highlighted terms are defined independent of the current configuration of the B-spline surface, and therefore are precomputed using Equation 3.

For the gradient and Hessian of membrane energy, we use deformation gradient as intermediates and apply chain rule:

$$\begin{aligned}\frac{\partial \Psi_{\text{mem}}}{\partial \mathbf{C}^{i,j}} &= \frac{\partial \Psi_{\text{mem}}}{\partial \mathbf{F}} \frac{\partial \mathbf{F}}{\partial \mathbf{C}^{i,j}}, \\ \frac{\partial^2 \Psi_{\text{mem}}}{\partial (\mathbf{C}^{i,j})^2} &= \left( \frac{\partial \mathbf{F}}{\partial \mathbf{C}^{i,j}} \right)^T \frac{\partial^2 \Psi_{\text{mem}}}{\partial \mathbf{F}^2} \frac{\partial \mathbf{F}}{\partial \mathbf{C}^{i,j}} + \frac{\partial \Psi_{\text{mem}}}{\partial \mathbf{F}} \frac{\partial^2 \mathbf{F}}{\partial (\mathbf{C}^{i,j})^2},\end{aligned}\tag{9}$$

where the second term for Hessian vanishes. We provide derivation of terms  $\partial \mathbf{F} / \partial \mathbf{C}^{i,j}$  and  $\partial \Psi_{\text{mem}} / \partial \mathbf{F}$ , and use the implementation of positive-semi-definite-projected Hessian given in Kim [2020] as proxy of  $\partial^2 \Psi_{\text{mem}} / \partial \mathbf{F}^2$ . This ensures that the energy Hessian  $\partial^2 \Psi_{\text{mem}} / \partial (\mathbf{C}^{i,j})^2$  is positive semi-definite, which is required for solving optimization time integration problem using backtracking line search.

Using the same indexing as in Equation 8, the entries in the gradient  $\partial \mathbf{F} / \partial \mathbf{C}^{i,j}$  are given by

$$\frac{\partial F_{\alpha\beta}}{\partial \mathbf{C}_{\gamma}^{i,j}} = \delta_{\alpha\gamma} \left( \frac{\partial N_{i,j}}{\partial u} \frac{\partial u}{\partial X_\beta} + \frac{\partial N_{i,j}}{\partial v} \frac{\partial v}{\partial X_\beta} \right),\tag{10}$$

where

$$\delta_{\alpha\gamma} = \begin{cases} 1, & \alpha = \gamma \\ 0, & \alpha \neq \gamma \end{cases},\tag{11}$$

and the gradient  $\partial \Psi_{\text{mem}} / \partial \mathbf{F}$  is given by the sum of its components:

$$\frac{\partial \Psi_{\text{mem}}}{\partial \mathbf{F}} = \frac{\partial \Psi_{\text{stretch}}}{\partial \mathbf{F}} + \frac{\partial \Psi_{\text{shear}}}{\partial \mathbf{F}},\tag{12}$$

where

$$\begin{aligned}\frac{\partial \Psi_{\text{stretch}}}{\partial \mathbf{F}} &= 2\mathbf{F} \left( \left( 1 - \frac{1}{\sqrt{I_5(\mathbf{e}_0)}} \right) \mu_{\text{st}0} \mathbf{e}_0 \mathbf{e}_0^T + \left( 1 - \frac{1}{\sqrt{I_5(\mathbf{e}_1)}} \right) \mu_{\text{st}1} \mathbf{e}_1 \mathbf{e}_1^T \right), \\ \frac{\partial \Psi_{\text{shear}}}{\partial \mathbf{F}} &= 2\mathbf{F} \mu_{\text{st}} (I_6 - \mathbf{e}_0^T \mathbf{e}_1) (\mathbf{e}_0 \mathbf{e}_1^T + \mathbf{e}_1 \mathbf{e}_0^T).\end{aligned}\tag{13}$$

## 2.2 Bending Energy

Recall that we use the quadratic bending model from Bergou et al. [2006], where the energy density is defined as

$$\Psi_{\text{bend}} = \frac{1}{2} \mu_{\text{bd}} H^2,\tag{14}$$

where  $H$  denotes the mean curvature. The mean curvature can be computed using the induced Laplace-Beltrami operator  $\Delta$  on the surface:

$$H^2 = \langle \Delta \phi, \Delta \phi \rangle = \left\langle \left( \frac{\partial^2 \phi}{\partial X_1^2} + \frac{\partial^2 \phi}{\partial X_2^2} \right), \left( \frac{\partial^2 \phi}{\partial X_1^2} + \frac{\partial^2 \phi}{\partial X_2^2} \right) \right\rangle.\tag{15}$$

To obtain the explicit formula for mean curvature, we first use parametric coordinates as intermediates and apply chain rule to compute the derivatives  $\partial^2 \phi / \partial X_1^2$ :

$$\phi_{11} = \phi_{uu} \mathbf{u}_1^2 + \phi_{vv} \mathbf{v}_1^2 + 2\phi_{uv} \mathbf{u}_1 \mathbf{v}_1 + \phi_u \mathbf{u}_{11} + \phi_v \mathbf{v}_{11},\tag{16}$$

where subscripts are used to denote derivatives (e.g.  $\phi_1 := \partial\phi/\partial X_1$ ,  $\phi_{11} := \partial^2\phi/\partial X_1^2$ , similar for  $u$  and  $v$ ). The highlighted first and second order derivatives are precomputed using Equation 3 and Equation 5. By symmetry we can similarly get  $\phi_{22}$ , and then have

$$\begin{aligned}\Delta\phi = & (u_1^2 + u_2^2)\phi_{uu} + (v_1^2 + v_2^2)\phi_{vv} + 2(u_1v_1 + u_2v_2)\phi_{uv} \\ & + (u_{11} + u_{22})\phi_u + (v_{11} + v_{22})\phi_v\end{aligned}\quad (17)$$

Denote the coefficients of  $\Delta\phi$  before control point  $C^{i,j}$  as  $c_{ij}$ , i.e. writing explicitly

$$c_{ij} = \sum_{(m,n) \in \mathcal{I}} \left( (u_1^2 + u_2^2) \frac{\partial^2 N_{m,n}}{\partial u^2} + (v_1^2 + v_2^2) \frac{\partial^2 N_{m,n}}{\partial v^2} + (u_{11} + u_{22}) \frac{\partial N_{m,n}}{\partial u} + (v_{11} + v_{22}) \frac{\partial N_{m,n}}{\partial v} + 2(u_1v_1 + u_2v_2) \frac{\partial^2 N_{m,n}}{\partial u \partial v} \right) \quad (18)$$

where  $\mathcal{I}$  denotes the index set of all control points, and the basis functions  $N_{i,j}$  are evaluated at the same position as  $\phi$ . The bending energy can be expressed using the control points as

$$\Psi_{\text{bend}} = \frac{1}{2} \mu_{\text{bd}} \sum_{(i,j),(k,\ell) \in \mathcal{I}} c_{ij} c_{k\ell} \left( \sum_{w \in \{x,y,z\}} C_w^{i,j} C_w^{k,\ell} \right) \quad (19)$$

Here  $w$  traverses all coordinate components in  $\mathbb{R}^3$ . The energy gradient and Hessian can then be computed as

$$\begin{aligned}\frac{\partial \Psi_{\text{bend}}}{\partial C_w^{i,j}} &= \frac{1}{2} \mu_{\text{bd}} \sum_{(k,\ell) \in \mathcal{I}} c_{ij} c_{k\ell} C_w^{(i,j)} \\ \frac{\partial^2 \Psi_{\text{bend}}}{\partial C_w^{i,j} \partial C_{w'}^{k,\ell}} &= \frac{1}{2} \mu_{\text{bd}} c_{ij} c_{k\ell} \delta_{ww'},\end{aligned}\quad (20)$$

where  $w, w' \in \{1, 2, 3\}$  are component indices. Here the Hessian of bending energy is independent of the control points, and therefore can be computed in advance.

### 3 Performance Optimization

We describe the key strategies used to optimize the runtime performance of our method. In subsection 3.1, we detail our Newton solver setup and analyze the runtime breakdown, highlighting the trade-offs introduced by switching from linear FEM to B-spline FEM. Then, in subsection 3.2, we present our optimized Hessian assembly strategy, which ensures the efficiency of each Newton iteration despite the increased stencil size from B-spline discretization.

#### 3.1 Solver Details

We minimize our incremental potential (IP) using a projected Newton method with backtracking line search to ensure global convergence [Li et al. 2020]. After solving for the search direction on the control point degrees of freedom (DoFs) using Cholesky factorization in each Newton iteration, we propagate the search direction to the linear triangle mesh vertices using the B-spline basis functions. Continuous collision detection (CCD) is then performed to determine a large feasible step size to initialize the backtracking line search, ensuring a monotonic decrease in the IP. The solver terminates once the norm of the Newton search direction becomes sufficiently small. We refer to [Li et al. 2020] for more algorithmic and implementation details.

To ensure positive definiteness and reduce computational cost, we lump the mass matrix by summing each row:

$$M_{(i,j)(i,j)}^{\text{lump}} = \sum_{(k,\ell) \in \mathcal{I}} M_{(i,j)(k,\ell)}, \quad (21)$$

while setting all off-diagonal entries to zero. Gravity forces and boundary conditions are handled similarly to standard FEM treatments [Li et al. 2024] and are omitted here for brevity.

In traditional linear FEM frameworks, such as Huang et al. [2024]; Li et al. [2021], solving the linear system typically dominates the runtime. Our B-spline FEM approach exhibits a different runtime profile, due to a new trade-off between system size and matrix sparsity: quadratic B-spline surfaces can capture comparable wrinkling behaviors with significantly fewer DoFs compared to linear triangle meshes (validated in the main paper), thereby reducing the linear system size. However, each quadrature point on the B-spline surface is influenced by up to nine control points, resulting in larger local stencils and a denser global Hessian matrix. Moreover, multiple quadrature points are required per element, further increasing the cost of matrix assembly. The main paper shows the timing breakdown per Newton iteration, illustrating that, without careful optimization, Hessian assembly can become even more expensive than the linear solve.

### 3.2 Fast Hessian Assembly

Constructing IP’s global Hessian matrix in compressed sparse column (CSC) format for the linear solver involves two main steps: 1) compute local Hessians at quadrature points and collect their entries as triplets (row, column, value); 2) assemble these triplets into a CSC matrix. Our reduced integration schemes already effectively accelerate step 1) by reducing the number of quadrature points and stencil sizes. For step 2), the `setFromTriplets` routine from Eigen [Guennebaud et al. 2010] is used, where runtime mainly depends on the number of triplets.

Triplet entries in the global Hessian originate from the local Hessians of both elasticity and contact energies. To accelerate the assembly of the elasticity Hessian, we focus on efficiently merging duplicate entries that share the same row and column indices prior to calling `setFromTriplets`. To enable this, we precompute a mapping from each control point to the set of quadrature points within its open support during simulation initialization. During assembly, we identify the control points associated with each global Hessian entry and merge the corresponding local Hessian contributions from their quadrature points in parallel. In the interior knot spans, each control point is associated with 12 quadrature points (see Figure 1). This parallel merging strategy reduces the number of triplet entries by a factor of 12, significantly improving the efficiency of matrix assembly.

For the contact Hessian derived from the linear triangle mesh, the sparsity pattern varies with the configuration and is not known in advance. However, similar optimization opportunities exist, as neighboring contact pairs often generate multiple triplets that correspond to the same Hessian entry. Moreover, as shown by the chain rule in the main paper, a single entry in the triangle mesh Hessian can contribute to up to 81 entries in the B-spline Hessian, since most points on the B-spline surface lie within the support of 9 control points. To avoid excessive growth in the number of Hessian entries during the tensor product expansion, we first assemble the triangle mesh Hessian into CSC format. We then apply the chain rule to compute the B-spline Hessian by traversing the nonzero entries, which is efficient for CSC.

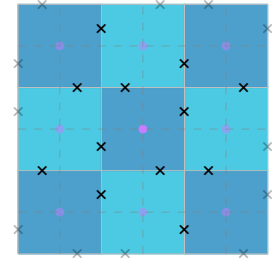

Fig. 1. **Mapping control point to quadrature points.** Example of an interior  $3 \times 3$  knot span. The example control point (purple dot) and its associated quadrature points ( $\times$ ) are highlighted.

#### 4 Additional Results

As stated in our paper, by applying our reduced integration scheme, we can significantly lower the computational cost for Hessian assembly, and improve the performance of linear solving. We now verify that this does not impair convergence of Newton method. As shown in Figure 2, under the same threshold, the reduced integration scheme requires similar number of iterations to convergence compared to the normal scheme, i.e.  $2 \times 2$  quadrature rule per knot span.

We further validate that it is necessary to have denser quadrature points for knot spans on the boundary. Below in Figure 3, we simulate a piece of cloth sheet laid flat, hanging on two of its corners on the same edge, and swinging due to gravity. Applying reduced integration uniformly on all knot spans or using  $2 \times 2$  rule on the corner both produce noticeable artifacts. Increasing the local quadrature order to  $3 \times 3$  largely mitigates the artifacts.

Table 1. **Simulation Statistics.** For cases involving contact, the resolution of the linear mesh used for collision handling is noted in parentheses. In contact-free simulations, B-spline FEM achieves up to a  $2\times$  speedup over linear FEM and a  $4\times$  speed up compared to second-order FEM (SFEM) [Le et al. 2023]. In contact-rich scenarios, our method maintains slightly better performance than linear FEM. All runtimes are reported as averages per timestep.

| Case                     | Method   | Resolution                            | Runtime (s) |
|--------------------------|----------|---------------------------------------|-------------|
| Upright Hanging Cloth    | B-spline | $75 \times 75$                        | 1.260       |
|                          | Linear   | $115 \times 115$                      | 2.953       |
|                          | B-spline | $100 \times 100$                      | 2.899       |
|                          | Linear   | $175 \times 175$                      | 7.815       |
|                          | B-spline | $125 \times 125$                      | 4.834       |
|                          | Linear   | $200 \times 200$                      | 10.962      |
| Drape Test               | B-spline | $100 \times 100$                      | 1.953       |
|                          | Linear   | $150 \times 150$                      | 3.754       |
|                          | B-spline | $125 \times 125$                      | 2.741       |
|                          | Linear   | $175 \times 175$                      | 5.614       |
|                          | SFEM     | $125 \times 125$                      | 21.351      |
| Shear Test               | B-spline | $100 \times 100$                      | 2.741       |
|                          | Linear   | $125 \times 125$                      | 5.614       |
|                          | B-spline | $125 \times 125$                      | 8.652       |
|                          | Linear   | $150 \times 150$                      | 15.622      |
|                          | B-spline | $140 \times 140$                      | 16.568      |
|                          | SFEM     | $125 \times 125$                      | 72.464      |
| Cloth On Sphere          | B-spline | $75 \times 75$ ( $85 \times 85$ )     | 3.098       |
|                          | Linear   | $85 \times 85$                        | 3.817       |
| Cloth On Bunny           | B-spline | $125 \times 125$ ( $175 \times 175$ ) | 18.46       |
| Cloth On Rotating Sphere | B-spline | $200 \times 200$ ( $300 \times 300$ ) | 357.84      |

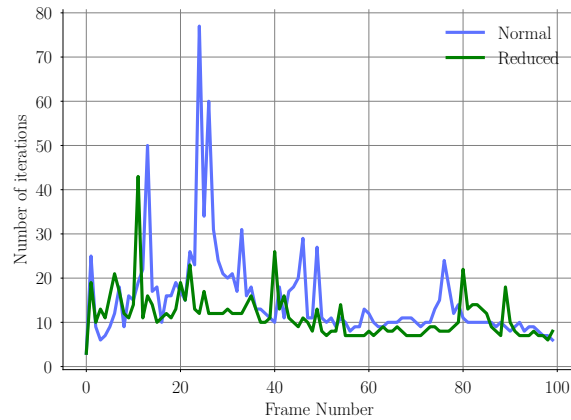

Fig. 2. **Newton Convergence with and without Reduced Integration.** Newton iteration counts over the first 100 timesteps of a hanging cloth simulation. The results show that reduced integration does not negatively impact the convergence rate of the Newton solver.

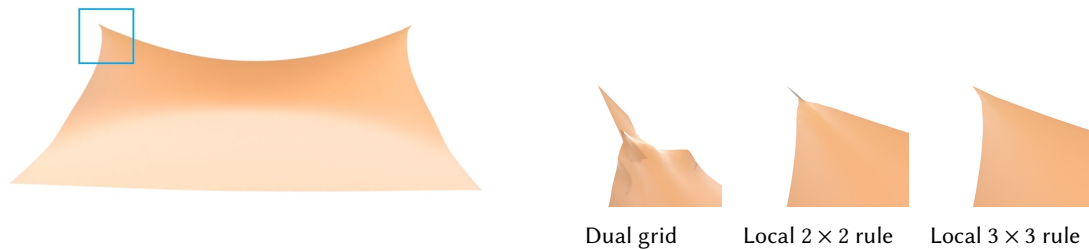

Fig. 3. **Quadrature Placement at Corners.** Left: Cloth hanging from two corner points undergoing deformation. Right: Zoom-in on the corner marked by the blue box, comparing different quadrature schemes. Dual grid one-point quadrature placement leads to severe tangling. Local  $2 \times 2$  quadrature reduces tangling but leaves noticeable artifacts. Local  $3 \times 3$  quadrature produces a smooth and physically plausible result.

## References

- Miklos Bergou, Max Wardetzky, David Harmon, Denis Zorin, and Eitan Grinspun. 2006. A quadratic bending model for inextensible surfaces. In *Proceedings of the Fourth Eurographics Symposium on Geometry Processing* (Cagliari, Sardinia, Italy) (SGP '06). Eurographics Association, Goslar, DEU, 227–230.
- Gaël Guennebaud, Benoît Jacob, et al. 2010. Eigen v3. <http://eigen.tuxfamily.org>.
- Kemeng Huang, Floyd M Chitalu, Huancheng Lin, and Taku Komura. 2024. GIPC: Fast and stable Gauss-Newton optimization of IPC barrier energy. *ACM Transactions on Graphics* 43, 2 (2024), 1–18.
- Theodore Kim. 2020. A Finite Element Formulation of Baraff-Witkin Cloth. *Computer Graphics Forum* 39, 8 (Nov. 2020), 171–179. <https://doi.org/10.1111/cgf.14111>
- Qiqin Le, Yitong Deng, Jiamu Bu, Bo Zhu, and Tao Du. 2023. Second-Order Finite Elements for Deformable Surfaces. In *SIGGRAPH Asia 2023 Conference Papers* (SA '23). ACM, 1–10. <https://doi.org/10.1145/3610548.3618186>
- Minchen Li, Zachary Ferguson, Teseo Schneider, Timothy Langlois, Denis Zorin, Daniele Panozzo, Chenfanfu Jiang, and Danny M. Kaufman. 2020. Incremental Potential Contact: Intersection- and Inversion-free Large Deformation Dynamics. *ACM Trans. Graph. (SIGGRAPH)* 39, 4, Article 49 (2020).
- Minchen Li, Chenfanfu Jiang, and Zhaofeng Luo. 2024. *Physics-Based Simulation*. <https://phys-sim-book.github.io/>

Minchen Li, Danny M Kaufman, and Chenfanfu Jiang. 2021. Codimensional incremental potential contact. *ACM Transactions on Graphics (TOG)* 40, 4 (2021), 1–24.
